# Supplementary material for: X-ResQ: Reverse Annealing for Quantum MIMO Detection with Flexible Parallelism
Source: arXiv:2402.18778 source file (2024-03-09)
Supplement: Supplementary file 1 [file QA_Appendix.tex]

\section{Scheduling of QA Algorithms: FA and RA}
\label{s:QA_apppendix}

On the machine hardware, $f_i$ is programmed on superconducting flux circuits or \emph{qubits}, while $g_{ij}$ is programmed on devices called \emph{couplers} by controlling local inductances. The time evolution of \emph{Hamiltonian} $\mathcal{H}$ in a system enables QA heuristics to solve the input optimization problem, where $\mathcal{H}$ can be defined as:
\begin{small}
\begin{align}
\mathcal{H}(\tau)
=A(\tau)\cdot\mathcal{H}_{\text{superposition}}+B(\tau)\cdot\mathcal{H}_{\text{problem}\,E}\notag\\
=A(\tau)\left(\sum_i \sigma_i^x\right) +B(\tau)\left(\sum_i f_{i} \sigma_i^z + \sum_{i<j} g_{ij} \sigma_i^z\sigma_j^z\right),
% =A(\tau)\cdot\mathcal{H}_{\text{superposition}}+B(\tau)\cdot E(\mathbf{s})
\label{eq:hamiltonian}
\end{align}
\end{small}

\noindent where $\tau$ is a time-dependent function ($\tau \in [0,1]$), while $\sigma^{x,z}$ are the Pauli matrices that represent the interaction of the spins, following the standard notation of quantum mechanics. How to control $\tau$ as a function of \emph{anneal duration} ($T_a$) 
% (\emph{i.e.,} how to do anneal scheduling) 
determines QA  algorithms. Figure~\ref{f:anneal_scheudle} shows two anneal signals as a function of $\tau$, where $A(\tau)$ represents the transverse energy that controls the strength of the \emph{quantum
fluctuations} (\emph{i.e.,} quantum-coherent exploration of the search
space), while $B(\tau)$ is the energy that is meant to correlate these fluctuations to the energy function of the problem (Eq.~\ref{eq:ising-ham}).

In the standard QA (called \emph{Forward Annealing} or FA), the system initially applies strong quantum fluctuations and prepares a \emph{quantum superposition state} that holds every possible configuration information (\emph{i.e.,} $A(\tau) \gg B(\tau)$ at $\tau=0$), and then drives the changes until the effect of the initial $\mathcal{H}_{\text{superposition}}$ diminishes (\emph{i.e.,} $A(\tau) \ll B(\tau)$ at $\tau=1$).\footnote{The state at $\tau=0$ indicates a fully quantum state, while the state at $\tau=1$ indicates a fully classical state.} During the anneal duration (user parameter range: $T_a \in$ [$0.5,2,000\,\mu$s]), $\tau$ increases incrementally from 0 to 1, hoping that adiabatic (or quasistatic~\cite{DWPauseMarshall}) nature of the thermodynamics will lead to a low-energy
state (a ground state in ideal cases), despite the noisy, imperfect implementation of the current hardware.

At the end of the anneal protocol, the $\sigma$ operators in Eq. \ref{eq:hamiltonian} can be identified to spin values, and 
the system can interpret the result as a classical spin state/configuration $\mathbf{s}$, being a \emph{sample}. Since QA is a probabilistic technique, the end result is non-deterministic. Thus, multiple runs of the solver ($N_a$ or \emph{anneal counts}) are typically applied, which will lead to $N_a$ configuration samples. Among them, the best sample $\mathbf{s}$ (\emph{i.e.,} min $E(\mathbf{s})$) is filtered as a final optimization solution. 
% Considering sequential runs of QA with its anneal duration (\emph{i.e.,} pure compute time: $N_a\times t_a$), 

\parahead{Reverse Annealing.} Contrary to FA, RA starts its processing from a classical state at $\tau=1$ (cf. a superposition state at $\tau=0$ in FA). For RA, the annealer initially programs a classical state on the hardware and then introduces quantum fluctuations 
by reducing $\tau$ to the \emph{switching point} $\tau_p$ ($0 \leq \tau_p \leq 1$ \emph{e.g.,} $\tau_p=0.4$~\cite{kim2020towards} or 0.6~\cite{pelofske2023initial}). When the process reaches the switching point, a superposition state is prepared with relatively weak fluctuations, which enables it to still hold the initial classical state information  After the optional pause ($P$), the rest of anneal duration follows the incremental increase of $\tau$ ($F$), like FA. 
Figure~\ref{f:anneal_algorithms} compares RA scheduling for $T_a=2.2~\mu$s w/ $\tau_p=0.4$ and $1~\mu$s pause used in \systemname{} (\S\ref{s:implementation}) against the FA scheduling for $T_a=1~\mu$s.

\begin{figure}
%\vspace*{4ex}
    \centering
    \begin{subfigure}[b]{0.49\linewidth}
    \centering
    %\raisebox{1ex}{\mbox{\includegraphics[width=\linewidth]{figures/DWH2.png}}}
    \includegraphics[width=\linewidth]{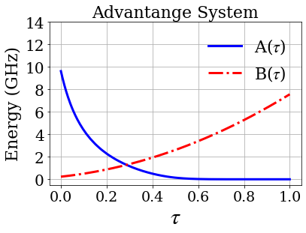}
    \caption{\footnotesize{Annealing signals across $\tau$.}}
    \label{f:anneal_scheudle}
    \end{subfigure}
    % \qquad
    \hfill
    \begin{subfigure}[b]{0.5\linewidth}
    \includegraphics[width=\linewidth]{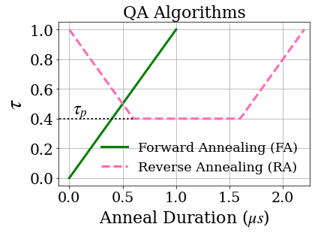}
    \caption{\footnotesize{Scheduling of QA Algorithms.}}
    \label{f:anneal_algorithms}
    \end{subfigure}

    % \begin{subfigure}[b]{\linewidth}\centering
    % \includegraphics[width=0.85\linewidth]{Figures/FA_RA.png}
    % \caption{Cost Landscape View.}
    % \label{f:rank_hdist}
    % \end{subfigure}
    
    % \begin{subfigure}[b]{\linewidth}
    % % \centering\includegraphics[width=0.8\linewidth]{Figures/RA_trade_off.png}
    % % \caption{\small{Optimization search properties of RA algorithms.}
    % %     % \caption{\small{Impact of the choice $\tau_p$ (switching point) on search in RA.}
    % % % Chance of leveraging the trade-off between exploitation and exploration in optimization existing in RA.
    % % }
    % % \label{f:expt_explr}
    % % \end{subfigure}
    
    \caption{\small\textbf{QA Signals and Algorithms. Figure~\ref{f:anneal_scheudle} shows annealing signals set on the D-Wave Advantage QA machine, while Figure~\ref{f:anneal_algorithms} plots signal controls for QA algorithms (FA and RA). Figure~\ref{f:expt_explr} illustrates RA's optimization search properties. 
    % depending on $\tau_p$ choice.
    }}
    % Pink dotted lines report the best cost/rank.
\label{f:annealing_background}
\end{figure}

Furthermore, it is noteworthy that the switching point $\tau_p$ determines the strength of applied quantum fluctuations. When $\tau_p$ is too far from the initial $\tau=1$ (\emph{i.e.,} $\tau_p$ close to 0), the information related to the initial state would be wiped out with strong fluctuations (\emph{i.e.,} no effects of using the initial state). On the other way, when $\tau_p$ is too close to the initial $\tau=1$, the strength of quantum fluctuations is not enough to trigger sufficient superposition (\emph{i.e.,} no effects of quantum search). In other words, RA provides a chance of exploring a trade-off in searching between exploration and exploitation as shown in Figure~\ref{f:expt_explr}. 
This makes the investigation of RA compelling in that the search capabilities even in near-future QA will remain limited (while being improved) due to the existing quantum decoherence and noise on the hardware. 

\parahead{Selection of QA Parameters.} The choice of QA parameters in \systemname{} such as anneal duration ($T_a$) and switching point ($\tau_p$) is decided by the brute-force exploration, following the same steps as the previous work~\cite{kim2019leveraging,kim2020towards}. Ideally, QA parameter settings can be optimized per instance, considering different initialization states. However, this is not practical due to the lack of theoretical means to acquire the best setting per instance. 
Thus, we use the empirically-obtained best-median setting (as stated in $\S$\ref{s:primer_ra}) across instances.

\begin{table}[htbp]
\begin{tiny}
% \begin{footnotesize}
\centering
\caption{D-Wave quantum annealers and features: D-Wave 2000Q (DW2Q) \& Advantage (DWAdv) machine.}
% \vspace{-0.3cm}
\begin{tabularx}{\linewidth}{*{5}{Y}}
\toprule
& \textbf{\scriptsize{DW2Q}} & \textbf{\scriptsize{DWAdv}} & \textbf{\scriptsize{DWAdv2}} \scriptsize{(prototype)} & \textbf{\scriptsize{DWAdv2}} \scriptsize{(full-size)}  \\ \midrule
%Access time & 26.647~ms\\
%Access overhead & 5.834~ms\\
\textbf{\scriptsize{Release Year}} &  \scriptsize{2017} & \scriptsize{2020} & \scriptsize{2022} &
\scriptsize{(exp)} \scriptsize{2024} \\
\textbf{\scriptsize{Topology}} & \scriptsize{Chimera} & \scriptsize{Pegasus} & \scriptsize{Zephyr} & \scriptsize{Zephyr} \\
\textbf{\scriptsize{Qubits}} & \scriptsize{2000+} & \scriptsize{5000+} & \scriptsize{500+} & \scriptsize{7000+} \\
\textbf{\scriptsize{Connectivity}} & \scriptsize{6} & \scriptsize{15} & \scriptsize{20} & \scriptsize{20} \\
% Connectivity & $\simeq$ 9000~$\mu$s\\
 % & $\simeq$ 300~$\mu$s\\
% Post processing & 445~$\mu$s \\
% \midrule
% $(N_t)$\\
% \bottomrule
% \toprule
% \multicolumn{6}{c}{\textbf{Dense Urban}}\\ 
% \multicolumn{3}{c}{\textbf{Downlink}} & \multicolumn{3}{c}{\textbf{Uplink}} \\\midrule
% \text{poor} & \text{medium} & good & \text{poor} & \text{medium} & good\\
% 5~dB & 12.5~dB  & 17.5~dB  & 5~dB  & 7.5~dB & 9~dB\\
\bottomrule

\end{tabularx}
% \vspace{-0.2cm}
\label{t:DWAVE}
\end{tiny}
\end{table}

\parahead{Hardware Programming.} Unlike Ising spin models, physical qubits on real hardware are rather sparsely connected. Thus, we need extra qubits to compile the Ising problem on the machine. This procedure is called \emph{hardware minor embedding}~\cite{choi2008minor}. We use the clique embedding technique that is designed to embed fully-connected graph models into sparse graphs, since our ML models are (nearly-)fully connected.
For each Ising model in the combined model ($\S$\ref{s:parallel_QA}), we apply the clique embedding.
